# Supplementary material for: Modality of Equilibration in Non-equilibrium Systems
Source: arXiv:1403.3237 source file (2014-03-13)

Modality of Equilibration in Non-equilibrium Systems

Supplementary Material

**Algorithm to generate continuous time data (Matlab2013) for Cu**:

```
load Cu_1st.dat; % 1st principal component
Ntotal=3000;     % total no of data in 1st component
Ngap=53;         % no of data
Neffective=800;
np=6;            % no of poles
nz=4;            % no of zeros
a=Cu_1st([Ngap:Ngap+Neffective-1]);
imp=[-1;zeros(Neffective-1,1)];%impulse
a_data=iddata(a,imp,Neffective);
tf_Cu=tfest(a_data,np,nz);
impulse(tf_Cu);
```

**1st principal components and their fittings by continuous time data generated with the help of system identification technique**:

Solid lines are the 1st principal components and dotted lines are their fittings.

Al(91.18%)

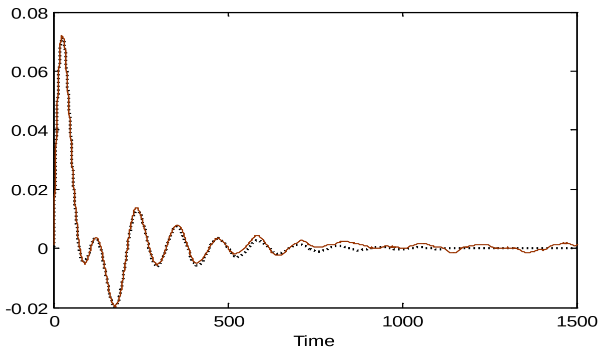


Cu(92.72%)

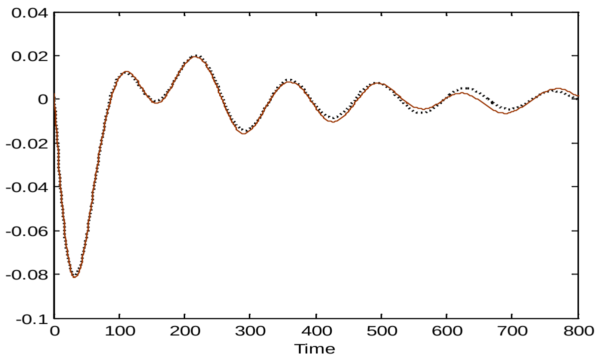

Fe(88.38%)

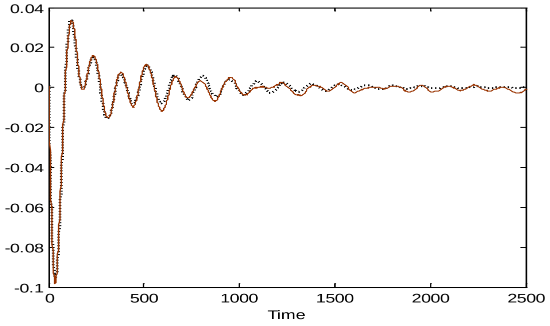


Solid Ar(95.59%)

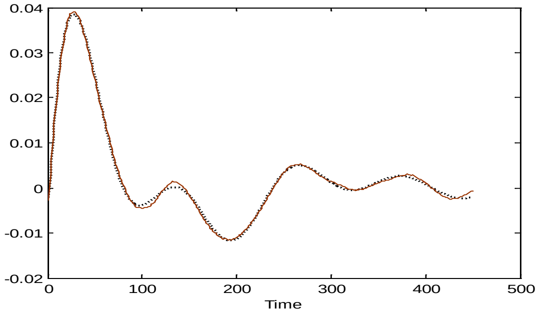


Si-500(82.31%)

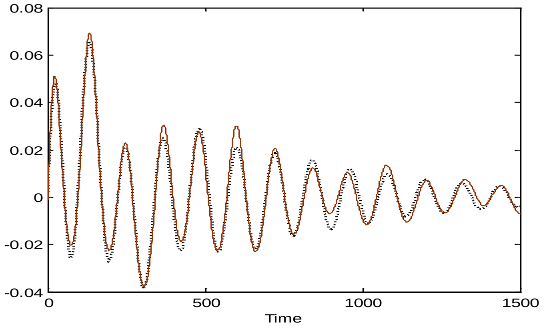


Si-800(81.45%)

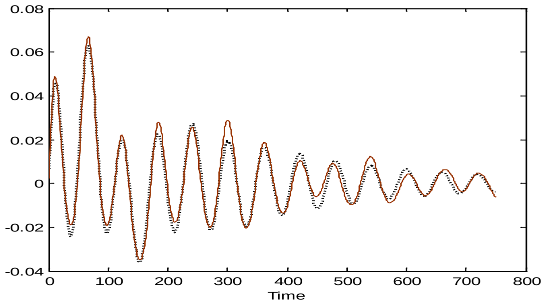

Ge-500(89.38%)

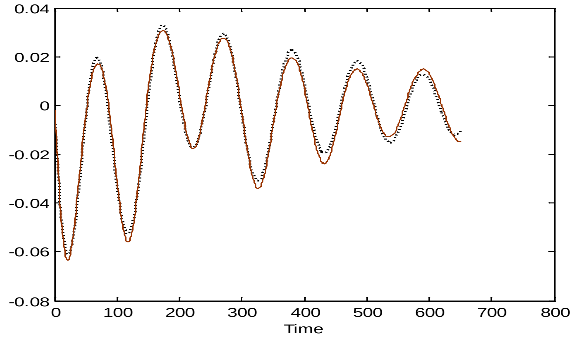


Ge-800(89.57%)

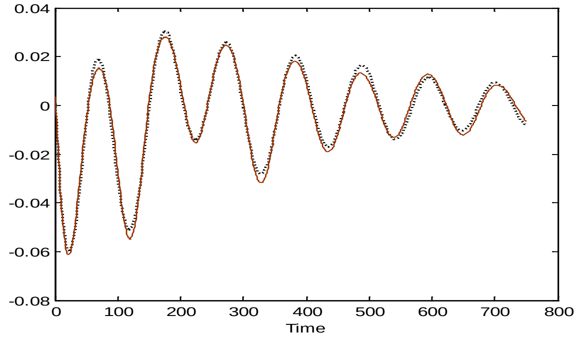


Mo(89.37%)

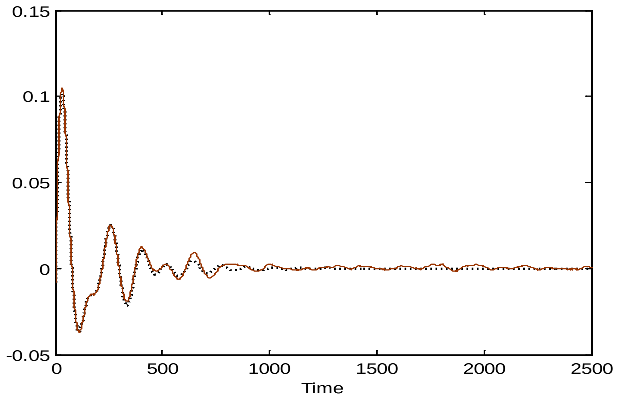

Supplement: Supplementary file 1 [file Supp_Modality_of_Equilibration.pdf]
